# Supplementary material for: Josephson Diode Effect Induced by Valley Polarization in Twisted Bilayer Graphene
Source: arXiv:2211.14846 source file (2023-12-14)

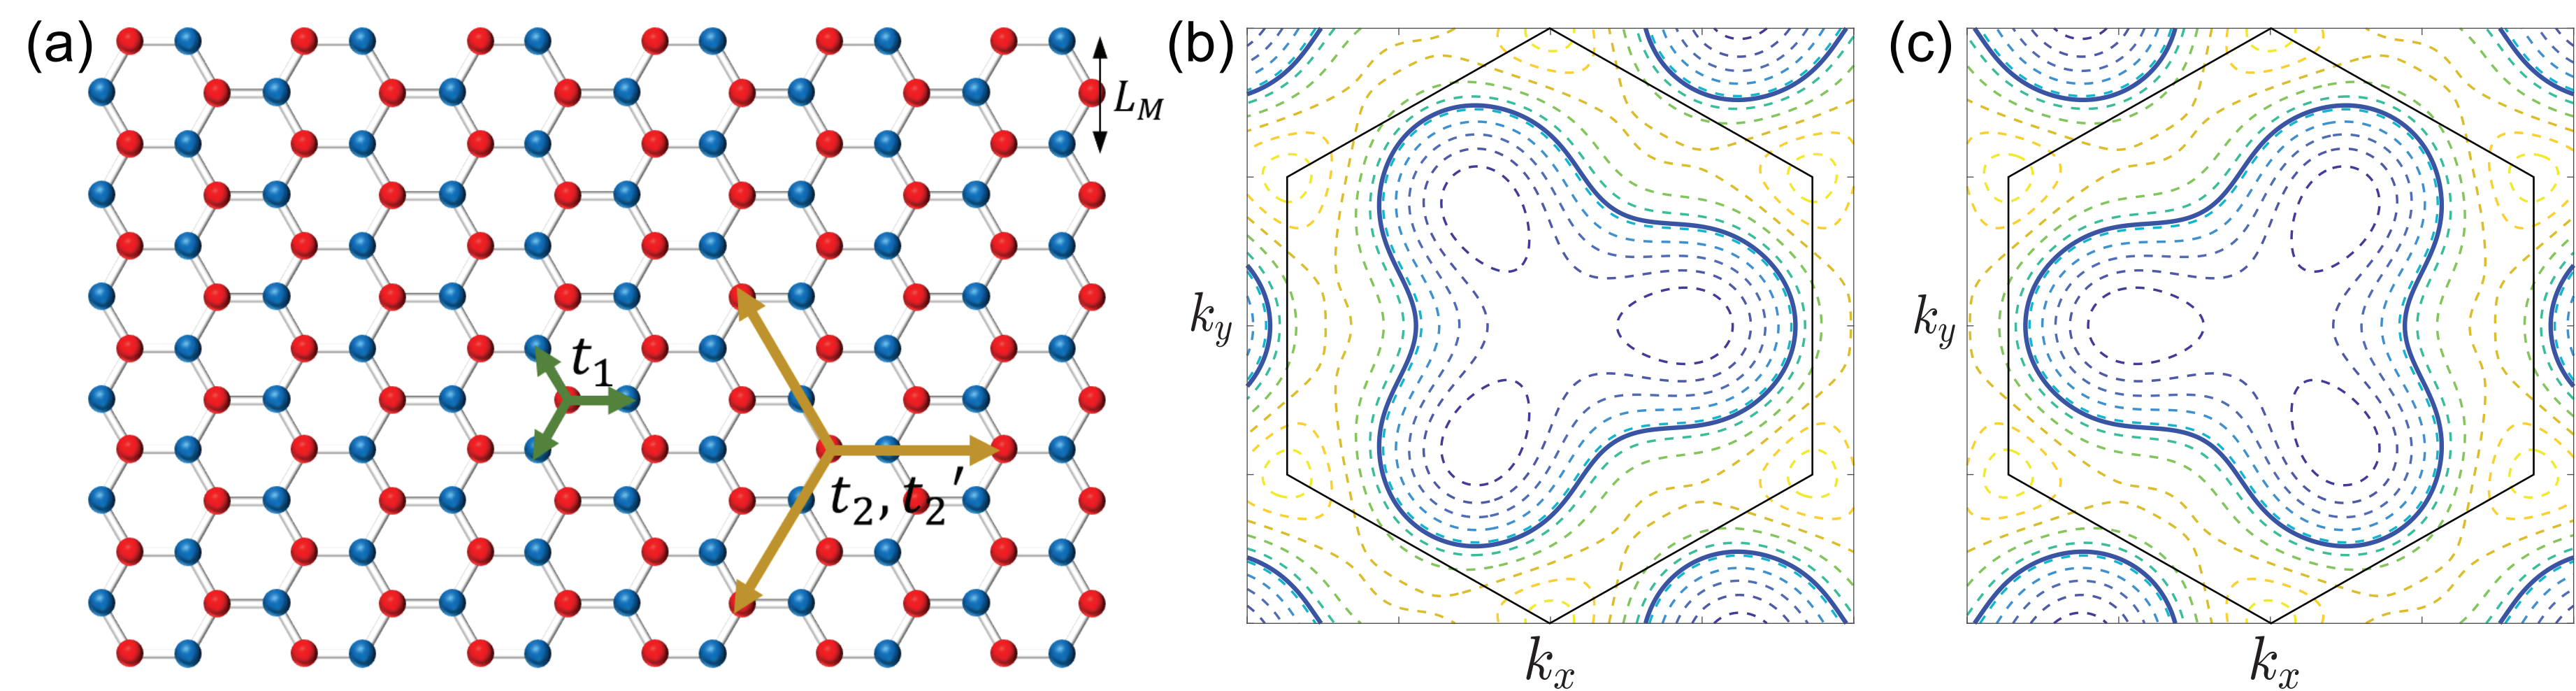

Supplement: Supplementary file 1 [file supple_figure2.pdf]
